# Supplementary material for: Infinite Texture: Text-guided High Resolution Diffusion Texture Synthesis
Source: arXiv:2405.08210 source file (2024-05-13)
Supplement: Supplementary file 1 [file 7_suppl.tex]

\appendix

\setcounter{figure}{0}

\setcounter{table}{0}

\section{Implementation Details}
\model is implemented in PyTorch~\cite{paszke2019pytorch}. All trainings used the AdamW optimizer~\cite{loshchilov2017decoupled} with default hyperparameters. All trainings ran on a single NVIDIA A100 GPU.

\subsection{Per-Texture Fine-tuning}
We fine-tune a diffusion model for each reference texture image. This is to learn the specific texture statistics of the reference texture. We initialize the diffusion model with the Stable Diffusion v2~\cite{rombach2021highresolution} checkpoint. For fine-tuning, we use a learning rate of $2e^{-6}$ with a batch size of $1$. The diffusion model is trained on random patches of size $768 \times 768$ for $1000$ iterations. It takes approximately $10$ minutes to fine-tune the diffusion model.

It is important to strike a balance during the fine-tuning phase. If fine-tuning is prolonged excessively, the learned image priors can be lost, and the model may overfit exclusively to the reference texture image. To address this, we choose to fine-tune for $1000$ iterations serves as a suitable middle ground. By adopting this approach, the fine-tuned diffusion model retains the capacity to generate diverse texture samples that resemble the reference texture, while benefiting from the preserved image prior.

\subsection{Texture Synthesis}
At inference time, we employ a deterministic DDIM~\cite{song2020denoising} sampler to iteratively denoise a noisy latent map. We use a total of $50$ time steps for the sampling process. At each time step, we randomly denoise patches of size $768 \times 768$ ($96 \times 96$ in the latent space) and then aggregate them by taking the average. We use a set of $90$ random patches, resulting in an output texture of size $2304 \times 2304$. This ensures that the entire image is covered $10$ times on average.
In contrast, the original MultiDiffusion~\cite{bar2023multidiffusion} uses a set of over $1000$ fixed patches. Our method achieves comparable visual quality while significantly improving the runtime by a factor of $10$. 
Once the latent code is denoised, Stable Diffusion use a decoder from VQGAN~\cite{esser2020taming} to transform the latent code into a color image. 
However, due to the large size of our latent code, it cannot be decoded all at once due to memory constraints.
Hence, we follow the same procedure described in Sec.~\ref{sec:multidiffison} 
to decode random patches and combine them by averaging to obtain the output color texture image.
It takes approximately $6$ minutes to iteratively denoise for $50$ steps and output a texture of size $2304 \times 2304$.

\subsection{Texture Transfer}
\begin{figure}[!t]
    \begin{center}

    \begin{subfigure}[t]{0.32\linewidth}
    \includegraphics[width=\linewidth]{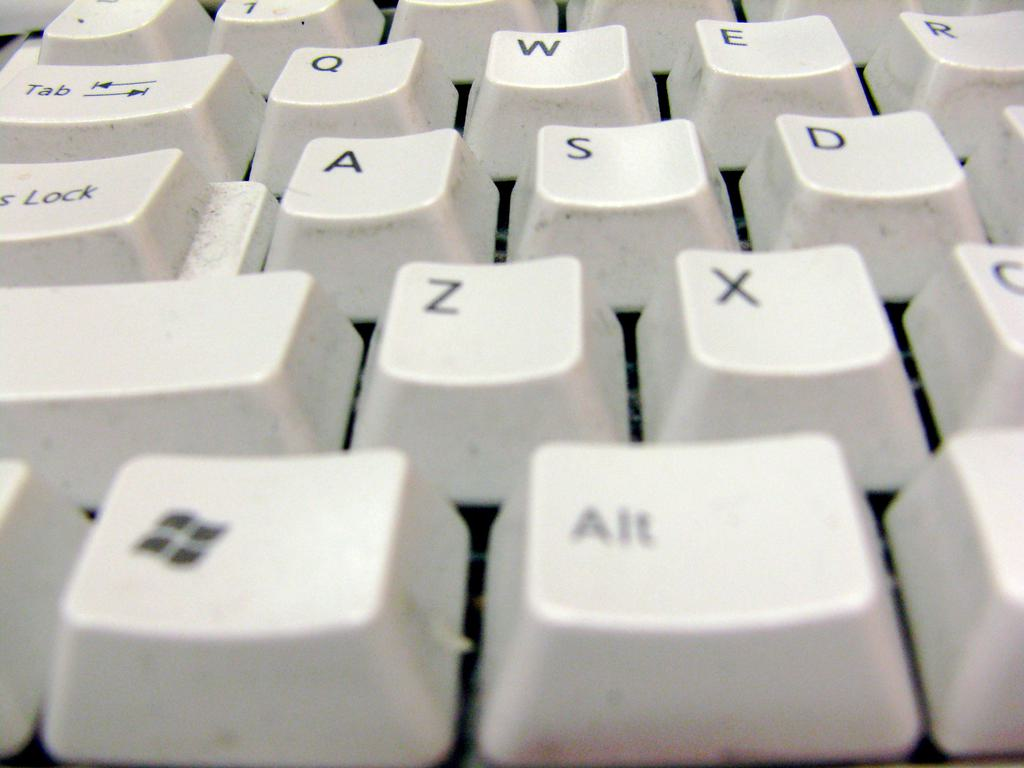} %
    \end{subfigure}
    \begin{subfigure}[t]{0.32\linewidth}
    \includegraphics[width=\linewidth]{fig/retexture/keyborard/control.png} %
    \end{subfigure}
    \begin{subfigure}[t]{0.32\linewidth}
    \includegraphics[width=\linewidth]{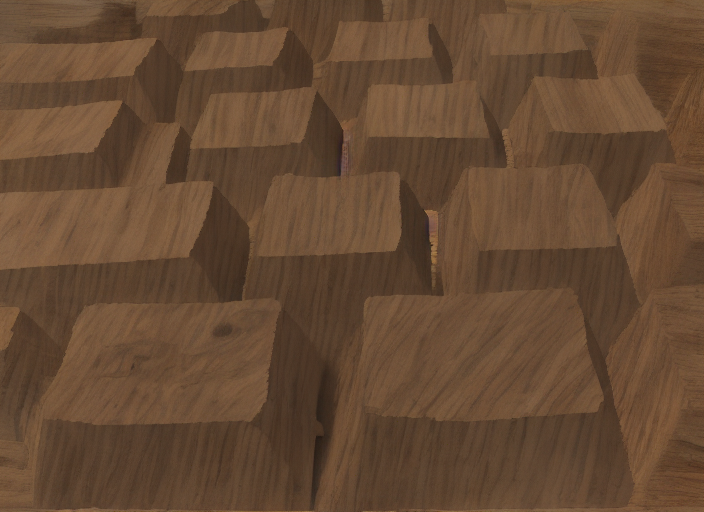} %
    \end{subfigure}\\

    \begin{subfigure}[t]{0.32\linewidth}
    \includegraphics[width=\linewidth]{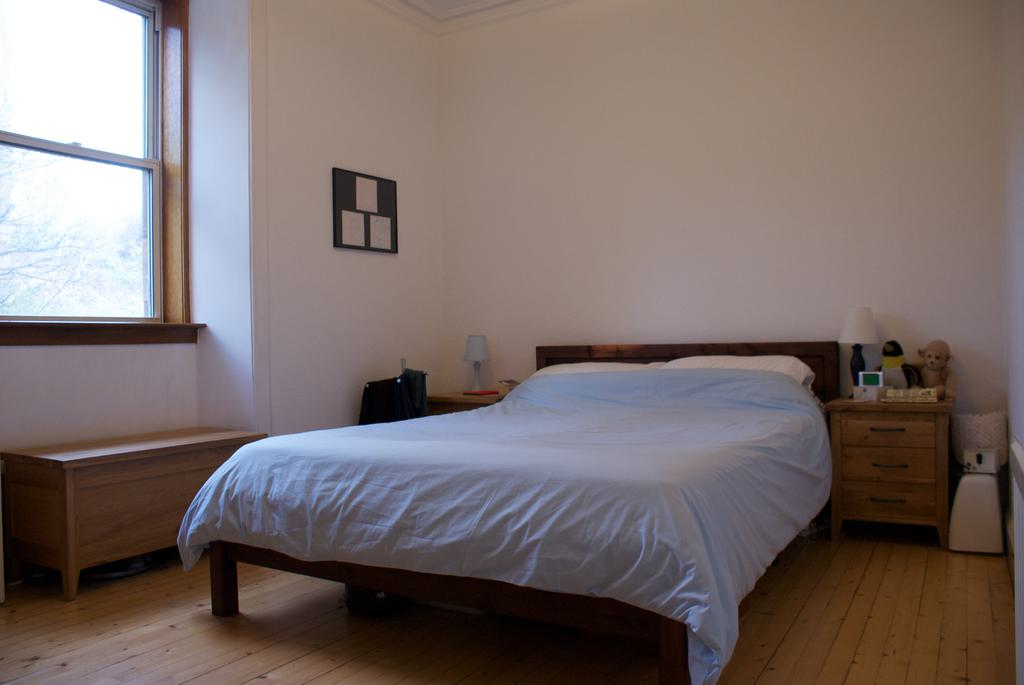} %
    \caption*{Input}
    \end{subfigure}
    \begin{subfigure}[t]{0.32\linewidth}
    \includegraphics[width=\linewidth]{fig/retexture/bedroom/control.png} %
    \caption*{ControlNet~\cite{zhang2023adding}}
    \end{subfigure}
    \begin{subfigure}[t]{0.32\linewidth}
    \includegraphics[width=\linewidth]{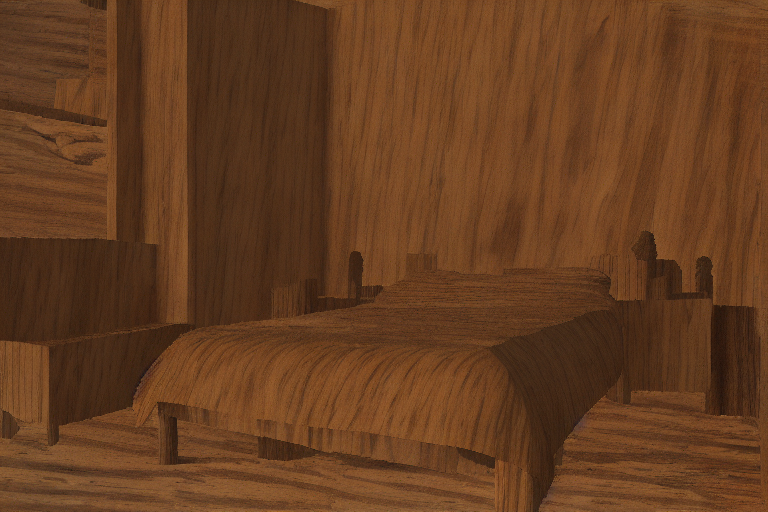} %
    \caption*{Ours}
    \end{subfigure}

    \caption{The vanilla ControlNet does not produce results with consistent texture with the input image and the reference texture. It also transfers the texture only to some regions of the image, not the entire image. Our results preserve the statistics of the input texture, while sharing consistent shading and shape with the input image.}
    \label{fig:retex_ab}
    \end{center}
\end{figure}

\begin{figure}[!t]
    \begin{center}

    \begin{subfigure}[t]{0.24\linewidth}
    \includegraphics[width=\linewidth]{fig/retexture/data/000.png} %
    \end{subfigure}
    \begin{subfigure}[t]{0.24\linewidth}
    \includegraphics[width=\linewidth]{fig/retexture/data/001.png} %
    \end{subfigure}
    \begin{subfigure}[t]{0.24\linewidth}
    \includegraphics[width=\linewidth]{fig/retexture/data/002.png} %
    \end{subfigure}
    \begin{subfigure}[t]{0.24\linewidth}
    \includegraphics[width=\linewidth]{fig/retexture/data/003.png} %
    \end{subfigure}\\

    \begin{subfigure}[t]{0.24\linewidth}
    \includegraphics[width=\linewidth]{fig/retexture/data/000_depth.png} %
    \end{subfigure}
    \begin{subfigure}[t]{0.24\linewidth}
    \includegraphics[width=\linewidth]{fig/retexture/data/001_depth.png} %
    \end{subfigure}
    \begin{subfigure}[t]{0.24\linewidth}
    \includegraphics[width=\linewidth]{fig/retexture/data/002_depth.png} %
    \end{subfigure}
    \begin{subfigure}[t]{0.24\linewidth}
    \includegraphics[width=\linewidth]{fig/retexture/data/003_depth.png} %
    \end{subfigure}

    \caption{Sample training data for texture transfer. We constructed a minimal dataset of $500$ image/depth pairs to fine-tune the ControlNet.}
    \label{fig:retex_data}
    \end{center}
\end{figure}

Texture transfer is a process where a given texture is applied to another image, guided by various properties of the latter. Our approach formulates texture transfer as an image synthesis task conditioned on scene depth. We leverage ControlNet~\cite{zhang2023adding} to transfer our generated textures to new surfaces.
Directly applying the ControlNet~\cite{zhang2023adding} on the estimated depth map performs poorly, as shown in Fig.~\ref{fig:retex_ab}. The vanilla ControlNet does not produce results with consistent texture and shading with the input image.
Instead, we fine-tune ControlNet on a minimal dataset constructed from texture-mapped primitives.
This allows it to generalize to nature images while maintaining consistent shading and shape with the input image.
In the following paragraphs, we provide more details about training data and scheme.

\subsubsection{Data}
We utilize the generated high-resolution $2304 \times 2304$ texture from \model as the ground truth texture. We apply this texture to the faces of a 3D cube object. Subsequently, we render $500$ image/depth pairs of size $512 \times 512$ while maintaining a fixed camera, a fixed directional light, and introducing random scale and rotation to the cube. 
This approach ensures consistent shading across all the training images. Additionally, the texture also serves as the background image. Fig.~\ref{fig:retex_data} illustrates examples of the training data.

\subsubsection{Training ControlNet}
The depth map serves as an additional input to model the desired mapping to the surface. The ControlNet is based on the Stable Diffusion. It creates a trainable copy of the Stable Diffusion model for the conditional input. The conditional signal is added back into the Stable Diffusion in the decoder via zero convolution layers. We use the same loss as in Eq.~\ref{eq:diffusion} 
to train both the ControlNet and the decoder part of the Stable Diffusion.

We follow the same training strategy to train the ControlNet --- fine-tuning instead of training from scratch. 
We initialize the ControlNet with a Depth v1.1 checkpoint. 
For fine-tuning, we use a learning rate of $2e^{-6}$ and a batch size of $4$. The diffusion model is trained on the rendered image/depth pairs for $1000$ iterations. It takes approximately $20$ minutes to fine-tune the ControlNet.

At test time, given an input image, we first use MiDaS~\cite{Ranftl2022} to estimate the depth map. Subsequently, we pass the depth map to the ControlNet for texture transfer. The process of transferring the appearance of the texture to the input image, for a resolution of $512 \times 512$, takes approximately $5$ seconds.

\section{Additional Evaluation Studies}
Here we delve into more details on baseline methods. 
We then provide an analysis of the runtime comparison. 
Finally, we showcase additional qualitative results.

\subsection{Baseline Comparisons}
In the following paragraphs, we provide the details about how we train and test the baseline models, as well as our analysis of these baseline results.

\textbf{Image Quilting}
As an early texture synthesis method, Image Quilting~\cite{efros2001image} is a patch-based approach. It involves tiling an example patch into a grid and utilizing dynamic programming to determine an optimal path for cutting through the overlapping regions, and ideally results in a seamless tile composed of the same patch. In our experiments, we utilized a $512 \times 512$ patch from the reference texture. The patch is tiled in a 5-by-5 grid with a $60$-pixel overlapping region to synthesize the final texture image. The synthesized texture is of size $2220 \times 2220$.

However, as illustrated in Fig.~\ref{fig:qualitative_suppl}, image quilting tends to produce noticeable repetitive patterns when working with high-resolution example texture patches. This limitation arises because the complexity of solving the dynamic programming problem increases with higher resolutions. Consequently, the method does not converge to a good minimum and instead generates repetitive patterns.

\textbf{Self Tuning Texture Optimization.}
While non-parametric method~\cite{efros2001image} struggled with real-world high-resolution textures, Self Tuning Texture Optimization (STTO)~\cite{kaspar2015self} is a fully automatic, self-tuning texture synthesis method. It extends Texture Optimization~\cite{kwatra2003graphcut} to accommodate textures with large-scale structures, repetitions, and near-regular structures. STTO is capable of self-tuning its various parameters and weights, thereby eliminating the need for manual adjustment on a case-by-case basis. Additionally, STTO employs a smart initialization strategy to improve the synthesis of regular and near-regular textures. In our experiments, we adopted the original implementation of STTO. It takes in a $512 \times 512$ exemplar texture as input, and synthesizes a texture of size $2048 \times 2048$.

As shown in Fig.~\ref{fig:qualitative_suppl}, STTO tends to produce results with broken structures. It often converges to solutions where a smooth patch is repeatedly used. This is because the initialization strategy it employs is limited to a single layer of translation symmetry. STTO also fails with textures containing large but unpronounced features (e.g., fabric and wood), due to the contour detector's inability to detect reliable edges.

\textbf{Periodic Spatial GAN}
Periodic Spatial GAN (PSGAN)~\cite{bergmann2017learning} is a texture synthesis method based on the Generative Adversarial Network (GAN). PSGAN extends the DCGAN~\cite{radford2015unsupervised} network structure by incorporating a spatially periodic signal generator to learn the statistical properties of the given texture image. We trained PSGAN using random $512 \times 512$ crops from the reference texture image. To accommodate the high-resolution input (vs. $256 \times 256$ in~\cite{bergmann2017learning}), we added an additional convolutional layer to both the generator and discriminator, resulting in an increased receptive field size of $250$. At test time, we provide the generator with a large noise image, and it outputs a $2048 \times 2048$ texture image.

However, as depicted in Fig.~\ref{fig:qualitative_suppl}, PSGAN struggles to capture the frequency of the texture image. This limitation can be attributed to two main factors: firstly, the receptive field of the network remains too small to capture the statistics within the texture adequately; and secondly, the periodic signal generator is not specifically designed to handle high-frequency signals in high-resolution textures.

\textbf{Non-stationary texture synthesis}
Non-stationary texture synthesis (NSTS)~\cite{zhou2018non} is the state-of-the-art method in texture synthesis. It uses a generative adversarial network based on CycleGAN~\cite{zhu2017unpaired}. The generator is trained to double the spatial extent of texture blocks extracted from the exemplar texture. 
Once trained, the fully convolutional generator is capable of expanding the size of the input texture image.
During training, we adhere to the procedure outlined in~\cite{zhou2018non}. The generator takes randomly cropped $128 \times 128$ patches from the example texture as input and double their size, generating corresponding $256 \times 256$ patches. The discriminator is trained to detect these generated $256 \times 256$ patches. 
At test time, we begin with a $512 \times 512$ crop of the reference texture image. Using the generator, we double the size twice, obtaining the final $2048 \times 2048$ output texture. 

As shown in Fig.~\ref{fig:qualitative_suppl}, NSTS generates visually pleasing textures but fails to accurately follow the distribution of the input texture. 
This limitation can be attributed to two key factors. Firstly, the fully convolutional generator is constrained by its limited receptive field, preventing it from capturing the complete statistics of the texture. Secondly, the network's exclusive training on small patches ($256 \times 256$) exacerbates the issue, leading to overfitting on low-frequency details.

\subsection{Runtime}
We present a breakdown of the runtime for each method in Tbl.~\ref{tbl:runtime}. Image Quilting~\cite{efros2001image}, an early texture synthesis method, runs on CPU only and does not require any training. The complexity of solving the dynamic programming problem increases with higher resolutions. It takes approximately $60$ minutes to generate a texture of size $2220 \times 2220$. 
STTO is an optimzation-based method that also runs on CPU only. It is capable of self-tuning its various parameters and weights. The runtime of STTO varies depending on the initialization. On average, it takes $21$ minutes to generate a texture of size $2048 \times 2048$. 
PSGAN~\cite{bergmann2017learning} is based on a small DCGAN network structure. 
Training typically takes around $2$ hours. At test time, it can generate a texture of size $2048 \times 2048$, but will not scale to an arbitrarily large texture image due to memory constraint. NSTS~\cite{zhou2018non} is based on a relatively large CycleGAN network structure. Although training images are small in size, it still requires approximately $5$ hours to fully converge.
Similar to PSGAN, NSTS faces limitations in scaling to arbitrarily large texture images due to memory constraints. 
\model takes approximately $10$ minutes for fine-tuning a diffusion model and an additional $6$ minutes to generate a $2304 \times 2304$ texture or $90$ minutes for $9216 \times 9216$. Once trained, \model can generate the same texture image with different variations and can scale to arbitrarily large images, with the only constraint being that the runtime increases quadratically with the output resolution.

\subsection{Additional Results}
In Fig.~\ref{fig:qualitative_suppl}, we show additional qualitative comparasions with image quilting~\cite{efros2001image}, STTO~\cite{kaspar2015self}, PSGAN~\cite{bergmann2017learning}, and NSTS~\cite{zhou2018non}. \model stands out by generating the most consistent textures with variations, while also being the fastest method for high-resolution textures. This is achieved through several key factors. Firstly, the large receptive field of the diffusion model effectively covers the entire $768 \times 768$ image, allowing it to capture global statistics. Additionally, fine-tuning the model from a Stable Diffusion checkpoint ensures that it inherits image priors, contributing to improved synthesis results. Furthermore, training on large image patches enables us to learn both low-frequency and high-frequency statistics within the texture image, leading to enhanced texture quality.

We further demonstrate high resolution results in Fig.~\ref{fig:full_1_suppl}, Fig.~\ref{fig:full_2_suppl} and Fig.~\ref{fig:full_3_suppl}. \model exhibits robustness in generating consistent textures at high resolutions. Unlike GAN-based methods, \model is based on a diffusion model that progressively denoises a noisy latent code. As a result, it avoids the occurrence of infamous color patterns commonly observed in GAN-generated textures.

\section{Limitations}
While \model outperforms its variants and baseline methods, there are several important limitations to consider, as illustrated in Fig.~\ref{fig:fail}.
Firstly, since we fine-tune the diffusion model from the Stable Diffusion v2 checkpoint, it inherits certain image priors. This can lead to automatic adjustments in the lighting of the texture image, resulting in color drift.
Secondly, in order to achieve fast inference, we denoise random patches during testing. As a result, \model may not perform well on textures with strong directional distributions, such as a regular grid pattern.

\begin{table*}[t]
    \centering
    \begin{tabular}{l|ccccc}
        & Image Quilting~\cite{efros2001image} & STTO~\cite{kaspar2015self} & PSGAN~\cite{bergmann2017learning} & NSTS~\cite{zhou2018non} & Ours \\
    \hline
    Training (min) & 0       &  0     & 120   & 300  & 10   \\
    Testing (min)  & 60      &  21    & 0     & 0    & 6    \\
    \hline
    Total (min)    & 60      &  21    & 120   & 300  & 16  
    \end{tabular}
    \caption{\textbf{Runtime breakdown for synthesizing high-resolution textures.} All models are trained on a single NVIDIA A100 GPU, except for image quilting and STTO which run on a high-performance CPU. Among all the methods, \model stands out as the fastest for generating high-resolution textures (\eg $2048 \times 2048$).}
    \label{tbl:runtime}
\end{table*}

\begin{figure*}[!htbp]
    \begin{center}

    \begin{subfigure}[t]{0.07\linewidth}
    \includegraphics[width=\linewidth]{fig/qualitative/cloth_01.png} %
    \end{subfigure}
    \begin{subfigure}[t]{0.18\linewidth}
    \includegraphics[width=\linewidth]{fig/qualitative/cloth_01-1.png} %
    \end{subfigure}
    \begin{subfigure}[t]{0.18\linewidth}
    \includegraphics[width=\linewidth]{fig/qualitative/cloth_01_stto.png} %
    \end{subfigure}
    \begin{subfigure}[t]{0.18\linewidth}
    \includegraphics[width=\linewidth]{fig/qualitative/cloth_01.jpg} %
    \end{subfigure}
    \begin{subfigure}[t]{0.18\linewidth}
    \includegraphics[width=\linewidth]{fig/qualitative/cloth_01_fake_1_B.png} %
    \end{subfigure}
    \begin{subfigure}[t]{0.18\linewidth}
    \includegraphics[width=\linewidth]{fig/qualitative/cloth_01_1000_ours.png} %
    \end{subfigure}\\

    \begin{subfigure}[t]{0.07\linewidth}
    \includegraphics[width=\linewidth]{fig/qualitative/cloth_02.png} %
    \end{subfigure}
    \begin{subfigure}[t]{0.18\linewidth}
    \includegraphics[width=\linewidth]{fig/qualitative/cloth_02-1.png} %
    \end{subfigure}
    \begin{subfigure}[t]{0.18\linewidth}
    \includegraphics[width=\linewidth]{fig/qualitative/cloth_02_stto.png} %
    \end{subfigure}
    \begin{subfigure}[t]{0.18\linewidth}
    \includegraphics[width=\linewidth]{fig/qualitative/cloth_02.jpg} %
    \end{subfigure}
    \begin{subfigure}[t]{0.18\linewidth}
    \includegraphics[width=\linewidth]{fig/qualitative/cloth_02_fake_1_B.png} %
    \end{subfigure}
    \begin{subfigure}[t]{0.18\linewidth}
    \includegraphics[width=\linewidth]{fig/qualitative/cloth_02_1000_ours.png} %
    \end{subfigure}\\

    \begin{subfigure}[t]{0.07\linewidth}
    \includegraphics[width=\linewidth]{fig/qualitative/granite_00.png} %
    \end{subfigure}
    \begin{subfigure}[t]{0.18\linewidth}
    \includegraphics[width=\linewidth]{fig/qualitative/granite_00-1.png} %
    \end{subfigure}
    \begin{subfigure}[t]{0.18\linewidth}
    \includegraphics[width=\linewidth]{fig/qualitative/granite_00_stto.png} %
    \end{subfigure}
    \begin{subfigure}[t]{0.18\linewidth}
    \includegraphics[width=\linewidth]{fig/qualitative/granite_00.jpg} %
    \end{subfigure}
    \begin{subfigure}[t]{0.18\linewidth}
    \includegraphics[width=\linewidth]{fig/qualitative/granite_00_fake_1_B.png} %
    \end{subfigure}
    \begin{subfigure}[t]{0.18\linewidth}
    \includegraphics[width=\linewidth]{fig/qualitative/granite_00_1000_ours.png} %
    \end{subfigure}\\

    \begin{subfigure}[t]{0.07\linewidth}
    \includegraphics[width=\linewidth]{fig/qualitative/wood_02.png} %
    \end{subfigure}
    \begin{subfigure}[t]{0.18\linewidth}
    \includegraphics[width=\linewidth]{fig/qualitative/wood_02-1.png} %
    \end{subfigure}
    \begin{subfigure}[t]{0.18\linewidth}
    \includegraphics[width=\linewidth]{fig/qualitative/wood_02_stto.png} %
    \end{subfigure}
    \begin{subfigure}[t]{0.18\linewidth}
    \includegraphics[width=\linewidth]{fig/qualitative/wood_02.jpg} %
    \end{subfigure}
    \begin{subfigure}[t]{0.18\linewidth}
    \includegraphics[width=\linewidth]{fig/qualitative/wood_02_fake_1_B.png} %
    \end{subfigure}
    \begin{subfigure}[t]{0.18\linewidth}
    \includegraphics[width=\linewidth]{fig/qualitative/wood_02_1000_ours.png} %
    \end{subfigure}\\

    \begin{subfigure}[t]{0.07\linewidth}
    \includegraphics[width=\linewidth]{fig/qualitative/leather_04.png} %
    \caption{Input}
    \end{subfigure}
    \begin{subfigure}[t]{0.18\linewidth}
    \includegraphics[width=\linewidth]{fig/qualitative/leather_04-1.png} %
    \caption{Image Quilting~\cite{efros2001image}}
    \end{subfigure}
    \begin{subfigure}[t]{0.18\linewidth}
    \includegraphics[width=\linewidth]{fig/qualitative/leather_04_stto.png} %
    \caption{STTO~\cite{kaspar2015self}}
    \end{subfigure}
    \begin{subfigure}[t]{0.18\linewidth}
    \includegraphics[width=\linewidth]{fig/qualitative/leather_04.jpg} %
    \caption{PSGAN~\cite{bergmann2017learning}}
    \end{subfigure}
    \begin{subfigure}[t]{0.18\linewidth}
    \includegraphics[width=\linewidth]{fig/qualitative/leather_04_fake_1_B.png} %
    \caption{NSTS~\cite{zhou2018non}}
    \end{subfigure}
    \begin{subfigure}[t]{0.18\linewidth}
    \includegraphics[width=\linewidth]{fig/qualitative/leather_04_1000_ours.png} %
    \caption{Ours}
    \end{subfigure}

    \caption{Additional comparisons with baseline methods in texture synthesis.}
    \label{fig:qualitative_suppl}

    \end{center}
\end{figure*}

\begin{figure*}[!htbp]
    \begin{center}

    \begin{subfigure}[t]{0.99\linewidth}
    \includegraphics[width=\linewidth]{fig/full/honeycomb_03_1000_ours.png} %
    \caption*{\textit{orthographic surface texture of a honeycomb}}
    \end{subfigure}

    \caption{Additional qualitative results of \model. It takes $90$ minutes to generate this $9216 \times 9216$ texture (85 MP).}
    \label{fig:full_1_suppl}

    \end{center}
\end{figure*}

\begin{figure*}[!htbp]
    \begin{center}

    \begin{subfigure}[t]{0.99\linewidth}
    \includegraphics[width=\linewidth]{fig/full/rock_01_1000_ours.png} %
    \caption*{\textit{overhead view of a field of small rocks}}
    \end{subfigure}

    \caption{Additional qualitative results of \model. It takes $90$ minutes to generate this $9216 \times 9216$ texture (85 MP).}
    \label{fig:full_3_suppl}

    \end{center}
\end{figure*}

\begin{figure*}[!htbp]
    \begin{center}

    \begin{subfigure}[t]{0.99\linewidth}
    \includegraphics[width=\linewidth]{fig/full/grass_00_1000_ours.png} %
    \caption*{\textit{a photo of grass texture}}
    \end{subfigure}

    \caption{Additional qualitative results of \model. It takes $25$ minutes to generate this $4608 \times 4608$ texture (21 MP).}
    \label{fig:full_2_suppl}

    \end{center}
\end{figure*}
